# Supplementary material for: Capillarity-Driven Flows at the Continuum Limit
Source: arXiv:1510.00411 source file (2015-10-01)
Supplement: Supplementary file 1 [file NanoFluidicsPaper_v12c_Supplemental.pdf]

# Supplemental Material for "Capillary-Driven Flows at the Continuum Limit"

Olivier Vincent,[1,*] Alexandre Szenicer,[1] and Abraham D. Stroock[1,2,†]

[1] *School of Chemical and Biomolecular Engineering, Cornell University, Ithaca, New York 14853, USA*
[2] *Kavli Institute at Cornell for Nanoscale Science, Cornell University, Ithaca, New York 14853, USA*

* orv3@cornell.edu
† ads10@cornell.edu

# I. EXPERIMENTAL

## A. Sample Fabrication and Caracterization

Details of the fabrication of porous silicon by HF anodization, of the etched microfluidic glass, and their assembly by anodic bonding can be found in Ref. [1] and its associated Supplemental Information. The cross-section areas of the serpentine channel ($a = 1.06 \times 10^{-9}\,\mathrm{m}^2$) and of the porous silicon layer ($A = 1.31 \times 10^{-7}\,\mathrm{m}^2$) were measured from scanning electron microscope (Zeiss Ultra 55 SEM) images.

$N_2$ porosimetry at 77.3K was performed on a separate fully porosified wafer not bonded to glass. Surface area $S_\mathrm{p}$ and pore volume $V_\mathrm{p}$ were determined from BET analysis, allowing to estimate a pore radius $r_\mathrm{p} = 2V_\mathrm{p}/S_\mathrm{p} = 1.4$ nm and the porosity $\phi = V_\mathrm{p}/V_\mathrm{tot} = 0.45$. BJH analysis allowed to estimate dispersity, showing a distribution peaked around $r_\mathrm{p} = 1.4$ nm with a typical half width at half maximum (hwhm) of 0.4 nm.

## B. Experimental Procedure

For imbibition experiments, the sample was evacuated for at least 24 hours, then quickly transferred into a transparent container with the liquid of interest. Time was measured from the moment at which the sample made contact with the liquid and images of the samples were recorded with time-lapse photography using 5-second intervals.

Drying experiments typically followed imbibition experiments, as the pores were then full of liquid. The serpentine-shaped reservoir was filled through the inlet hole with the liquid using the following procedure : 1) evacuation for 1 minute to remove air from the reservoir, 2) dipping the sample in the liquid while still under vacuum, 3) venting the vacuum chamber. In step 3), the outside air pressure was sufficient to push the liquid into the reservoir and fill it completely without bubbles. Using an air blower above the inlet hole, part of the liquid was evaporated from the back of the serpentine channel to allow for the creation of a visible air-water meniscus in the channel. In order to prevent further evaporation of the liquid from the backside of the sample, the inlet hole was then sealed with at least 6 layers of stretched parafilm. The success of the sealing procedure was checked by exposing the sealed inlet to air for at least one hour and verifying that the meniscus motion was negligible.

In order to start a drying experiment, the sample was then transferred into a closed chamber. Relative humidity in the chamber was controlled by unsaturated aqueous solutions of NaCl or LiCl calibrated using Decagon WP4C water potential meter. For drying with liquids other than water, samples were exposed to ambient air which contains only traces of the solvents' vapors. This situation placed the system into the "plateau-drying" regime associated with low relative humidities (large, negative liquid potentials, see Fig. 2c in the Letter, regime ②).

During drying, the motion of the meniscus in the serpentine-shaped reservoir was recorded by time-lapse photography using 10-second intervals. We note here that the presence of a meniscus in the serpentine channel was associated with a capillary pressure on the order of $\sigma/H \simeq 4$ kPa where $H = 20\,\mu$m is the depth of the microchannel. We have neglected this capillary pressure in our analysis, the driving forces generated by drying being on the order of $10-100$ MPa in our system.

## C. Analysis

We performed the analysis of the drying experiments by measuring manually on the time-lapse images the position $X(t)$ of the meniscus in the serpentine channel, leading to the data in Fig. 2a-b in the Letter. We obtained the steady-state velocity $v$ and its associated uncertainty $\Delta v$ by linear fitting of the data for $t > 10 \times \tau_\mathrm{poro} = 18$ min to ensure sufficient decay of the poroelastic transient (see section III). We used the relation $J = (a/A) \times v$ to calculate the Darcy velocity $J$ of the fluid in the porous layer for the plot in Fig. 2c, propagating the uncertainty $\Delta v$. We also calculated the error bars on the driving force $\Psi_\mathrm{ext}$ by propagating through Kelvin equation $\Psi_\mathrm{ext} = (RT/v_\mathrm{m})\ln(p_\mathrm{ext}/p_\mathrm{sat})$ the uncertainty of $\pm 0.003$ on the activity $p_\mathrm{ext}/p_\mathrm{sat}$ imposed by the salt solutions as measured by Decagon WP4C water potential meter. Uncertainties on the cross sections $a$ and $A$ introduce an additional systematic error that we estimated to be $\pm 4\%$. We propagated that error on the final result for the permeability leading to $\kappa = (1.87 \pm 0.08) \times 10^{-17}\,\mathrm{m}^2/(\mathrm{Pa.s})$.

For the analysis of imbibition dynamics, we extracted the position of the wetting front $Y(t)$ by image analysis using the following procedure. We note $I_n(y', z)$ the gray-level intensity matrix of the $n^\mathrm{th}$ image in the time-lapse set, with $z$ corresponding to an axis perpendicular the the direction of propagation of the front, and $y'$ to an axis parallel to it (with opposite direction compared to the $y$ axis defined on Fig. 1 in the Letter, and origin at the edge of the sample, in other words $y' = L - y$). We use the first image of the set ($n = 0$) as a reference image to calculate the relative intensity change in the direction of propagation $\xi_n(y') = \langle (I_0 - I_n)/I_0 \rangle_z$ for every other image $n$, where $\langle\rangle_z$ represents

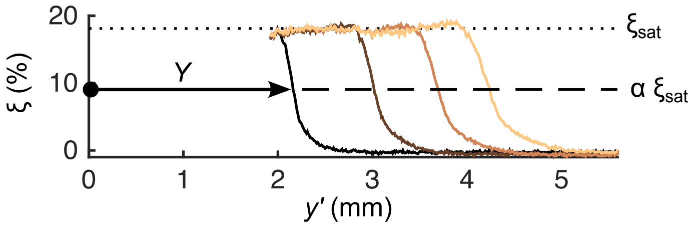


FIG. S1. Analysis of imbibition dynamics. $\xi(y)$ represents the relative intensity change along the direction of front propagation. Colors correspond to a subset of images that are 700 s apart during the experiment. The black dashed line corresponds to $\xi = \alpha\xi_{\mathrm{sat}}$ with $\alpha = 0.5$ and $Y$ is the extracted front position for the first $\xi(y)$ curve. See text for details.

TABLE S1. Physical parameters for the different liquids used. All values from Ref. [3] except the viscosity of isopropanol [4] and the contact angle values (measured, see section I D). Uncertainties on the molecular size are less than 0.13%.

| | Surface Tension $\sigma$ [mN/m] | Viscosity $\eta$ [mPa.s] | Molar Volume $v_{\mathrm{m}}$ [$\times 10^{-5}$m$^3$/mol] | Molecular size $(v_{\mathrm{m}}/\mathcal{N}_{\mathrm{A}})^{1/3}$ [nm] | Contact Angle $\theta$ [°] |
|---|---|---|---|---|---|
| Water | $72.4 \pm 0.6$ | $0.946 \pm 0.056$ | $1.806 \pm 0.001$ | 0.311 | $25 \pm 5$ |
| Acetone | $23.0 \pm 0.5$ | $0.315 \pm 0.009$ | $7.377 \pm 0.028$ | 0.497 | 0 |
| Ethanol | $22.2 \pm 0.4$ | $1.145 \pm 0.071$ | $5.848 \pm 0.021$ | 0.460 | 0 |
| Isopropanol | $21.1 \pm 0.4$ | $2.242 \pm 0.172$ | $7.664 \pm 0.028$ | 0.503 | 0 |

averaging over the direction perpendicular to the front propagation. A typical subset of generated $\xi_n(y')$ curves for an experiment is shown in Fig. S1. These curves transition from $\xi = 0$ where the porous silicon is dry to a positive value $\xi_{\mathrm{sat}}$ where it is saturated with liquid. We extracted the average front position $Y$ by searching each curve for the location where $\xi = \alpha\xi_{\mathrm{sat}}$. The data of Fig. 3a in the Letter was obtained using $\alpha = 0.5$ (main, black curve). Further, we used $\alpha = [0.25; 0.75]$ to evaluate a typical uncertainty on the front position (grey dotted lines on Fig. 3a).

### D. Liquid properties

Tabulated values of the viscosities and surface tensions of the bulk liquids were used for $\eta$ and $\sigma$ with an uncertainty estimated from the temperature dependence of these properties in the range $20 - 25$°C (Table S1 columns 1 and 2). The molecular sizes were computed from the tabulated bulk molar volumes using $d = (v_{\mathrm{m}}/\mathcal{N}_{\mathrm{A}})^{1/3}$ (Table S1 columns 3 and 4). Finally, contact angles were measured using the sessile drop method: organic liquids always showed complete spreading ($\theta = 0$) while we measured $\theta = 25 \pm 5°$ for water (Table S1 column 5), in agreement with values from the literature [2].

We neglected the dependence of the molar volumes on the liquid pressure. An order of magnitude of the relative variations of $v_{\mathrm{m}}$ can be obtained through $\Delta v_{\mathrm{m}}/v_{\mathrm{m}} = \chi_{\mathrm{liq}}\Delta P$ where $\chi_{\mathrm{liq}}$ is the liquid isothermal compressibility and $\Delta P$ the pressure variation. Using the maximum driving forces $\Delta P_{\mathrm{max}} \simeq 100$ MPa obtained with water ($\chi_{\mathrm{w}} = 4.5 \times 10^{-10}$ Pa$^{-1}$, we estimate $(\Delta v_{\mathrm{m}}/v_{\mathrm{m}})_{\mathrm{max}} \simeq 4.5\%$. In fact, using the International Association for the Properties of Water and Steam (IAPWS) equation of state for water, we find that the error in the liquid pressure estimated from Kelvin equation when assuming $v_{\mathrm{m}}$ constant is $< 1\%$ at $\Psi = -50$ MPa and 2.6% at $\Psi = -100$ MPa.

## II. STEADY-STATE DRYING MODEL

### A. Single pore

Here we consider drying-induced permeation through a hypothetical single straight cylindrical pore of length $L$ and of radius $r_{\mathrm{p}}$ (see Figs. 2d-e in the Letter), characterized by an intrinsic capillary pressure $\Psi_{\mathrm{c}} = -2\sigma\cos\theta/r_{\mathrm{p}}$. We assume that $\theta$ is the equilibrium contact angle, thus neglecting contact angle hysteresis effects.

One edge of the pore ($x = 0$) is in contact with a bulk reservoir of liquid so that $\Psi_{x=0} = 0$ in the pore liquid while the other edge is in equilibrium with the vapor pressure $p_{\mathrm{ext}}$ imposed outside of the sample so that $\Psi_{x=L} = \Psi_{\mathrm{ext}}$ with $\Psi_{\mathrm{ext}} = RT/v_{\mathrm{m}}\ln(p_{\mathrm{ext}}/p_{\mathrm{sat}})$ (Eq. (1) in the Letter).

- If $\Psi_{\rm ext} \geq \Psi_{\rm c}$, the pore remains completely filled with liquid. The meniscus is located in $x = L$ and adopts a radius of curvature $r$ set by the external relative humidity through Kelvin equation (Eq. (2) in the Letter) and Laplace equation $P_{\rm edge} - P_0 = -2\sigma/r$. The capillary stress, of magnitude $P_{\rm edge} - P_0 = \Psi_{\rm ext}$ results in a pressure-driven viscous flow proportional to $\Psi_{\rm ext}$. The resulting mass flux per unit area $q$ [kg/(m$^2$.s)] in the pore liquid (i. e. mass flux divided by $\pi r_{\rm p}^2$ the cross-section area of the pore) is

$$q = \frac{-\Psi_{\rm ext}}{L/g_{\rm liq}} = \frac{-\Psi_{\rm ext}}{R} \tag{S1}$$

  where we have defined the linear mass conductivity of a liquid-filled pore $g_{\rm liq}$ and the total mass transport resistance of the liquid-filled pore $R = \Delta\Psi/q = L/g_{\rm liq}$.

- If $\Psi_{\rm ext} < \Psi_{\rm c}$, mechanical capillary equilibrium at the pore end cannot be satisfied anymore. The meniscus recedes within the pore to a location $x = L - \epsilon$ so that $\Psi(L-\epsilon) = \Psi_{\rm c}$ for mechanical equilibrium to be satisfied again. Mass transport is thus determined by a succession of liquid transport on a distance $L - \epsilon$, and vapor transport on a distance $\epsilon$. There are now two mass transport resistances in series $R_{\rm liq} = (L-\epsilon)/g_{\rm liq}$ and $R_{\rm vap} = \epsilon/g_{\rm vap}$. The liquid potential drops being imposed in each phase ($\Delta\Psi_{\rm liq} = -\Psi_{\rm c}$ and $\Delta\Psi_{\rm vap} = \Psi_{\rm c} - \Psi_{\rm ext}$), a single value of $\epsilon$ leads to a unique mass flux ($\Delta\Psi_{\rm vap}/R_{\rm vap} = \Delta\Psi_{\rm liq}/R_{\rm liq}$), as required by the steady-state situation, satisfying $\epsilon/(L-\epsilon) = \Delta\Psi_{\rm vap}/\Delta\Psi_{\rm liq} \times (g_{\rm vap}/g_{\rm liq})$, or

$$\frac{\epsilon}{L-\epsilon} = \frac{\Psi_{\rm c} - \Psi_{\rm ext}}{-\Psi_{\rm c}} \times \beta. \tag{S2}$$

  The distance from the edge at which the meniscus recedes, $\epsilon$, thus scales as the ratio of conductances, $\beta = g_{\rm vap}/g_{\rm liq}$ which we now estimate. Assuming Poiseuille flow in the liquid-filled pore, $g_{\rm liq} = \rho r_{\rm p}^2/(8\eta)$ where $\rho$ is the liquid density. Assuming diffusion in the vapor phase, $q = \frac{M}{RT} D \frac{\Delta p}{\epsilon}$ where $M = \rho v_{\rm m}$ is the species molar mass, $D$ is the vapor diffusivity, and $\Delta p$ is the vapor pressure drop, related to the liquid potential drop $\Delta\Psi_{\rm vap}$ through Kelvin equation. Thus $g_{\rm vap} = (\Delta p/\Delta\Psi_{\rm vap}) \times MD/(RT)$. From Kelvin equation, $\Delta\Psi_{\rm vap}/\Delta p \simeq RT/(v_{\rm m} p_{\rm ext})$. We further assume Knudsen diffusion for the vapor [5]: $D = (2r_{\rm p}/3) \times (8RT/\pi M)^{1/2}$. We eventually find

$$\beta \simeq \frac{32}{3}\left(\frac{2}{\pi}\right)^{1/2}\left(\frac{RT}{M}\right)^{-3/2}\frac{\eta\, p_{\rm ext}}{\rho^2 r_{\rm p}}. \tag{S3}$$

  For water, taking a typical value of the vapor pressure $p_{\rm ext} = 1$ kPa, we find $\beta \simeq 10^{-4}$ with $r_{\rm p} = 1.7$ nm. We deduce from eq. (S2), that $\epsilon/L \ll 1$. This conclusion is unaffected when taking into account the negative slip length $\delta < 0$ for the flow of the liquid in the pores (resulting in a correction factor on $\beta$ of $(1+\delta/r_{\rm p})^{-4} \simeq 2$ for water and $\simeq 4$ for the organic liquids). Similarly, taking into acount the tortuosity $\tau$ of the pores does not affect the result, as vapor and liquid transport are affected in the same way (flux divided by $\tau$).

In the following we assume $\beta = 0$ (and thus $\epsilon = 0$), which results in the simple expression for the mass flux in a single pore of radius $r_{\rm p}$:

$$\begin{cases} q = -g_{\rm liq}\Psi_{\rm ext}/(\tau L) & \text{if } \Psi_{\rm ext} \geq \Psi_{\rm c} = -2\sigma\cos\theta/r_{\rm p} \\ q = -g_{\rm liq}\Psi_{\rm c}/(\tau L) & \text{if } \Psi_{\rm ext} < \Psi_{\rm c} \end{cases} \tag{S4}$$

where we have introduced the factor $\tau$ to take into account the tortuosity of the pores. Assuming that the porous medium is constituted of identical pores of radius $r_{\rm p}$, the two-parts response described in (S4) for a single pore naturally extends to the whole medium, resulting in regimes ① and ② described in the Letter.

### B. Pore size distribution

We now evaluate the effects of pore size distribution on the conclusions drawn above and in the Letter, which were based on the assumption that all pores have the same radius. For simplicity, we assume that the porous medium is constituted of a bundle of non-interacting cylindrical pores, each pore $i$ having a radius $r_i$. Under this assumption, the total mass flow rate $Q$ [kg/s] in the porous medium is the sum of the flow rates from all individual pores, following Eq. (S4).

$$Q = -\frac{1}{\tau L}\sum_i \Psi_i \times g_{{\rm liq},i} \times \pi r_i^2 \tag{S5}$$

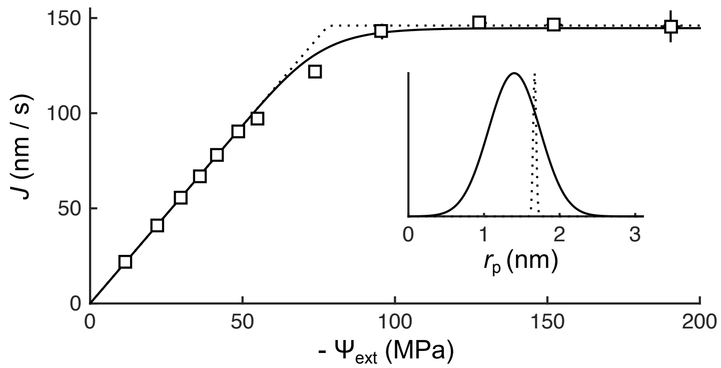


FIG. S2. Effect of the pore size distribution on the drying response. Full line correspond to a gaussian distribution or average radius 1.4 nm and hwhm of 0.4 nm (see inset) while the dotted line corresponds to a sharp distribution around 1.7 nm. The square data points represent the experimental results from Fig. 2c in the Letter.

with $g_{\mathrm{liq},i} = \rho(r_i+\delta)^4/(8\eta r_i^2)$, $\Psi_i = \Psi_{\mathrm{ext}}$ if $\Psi_{\mathrm{ext}} > \Psi_{\mathrm{c},i} = -2\sigma\cos\theta/r_i$ and $\Psi_i = \Psi_{\mathrm{c}}, i$ otherwise. Using the relation $Q = \rho A J$ and the definition of porosity $\phi = \sum \pi r_i^2/A$, we obtain the volumetric flux

$$J = -\frac{\phi}{8\eta\tau L}\frac{\left\langle \Psi_i \times (r_i+\delta)^4\right\rangle}{\langle r_i^2\rangle} \tag{S6}$$

where $\langle\rangle$ is the ensemble average over all pores. It is useful to consider the limiting case for low values of $-\Psi_{\mathrm{ext}}$ where $\Psi_i = \Psi_{\mathrm{ext}}$ for all pores (Kelvin-Darcy regime ①). The flux is then

$$J_1 = -\kappa\frac{\Psi_{\mathrm{ext}}}{L} \tag{S7}$$

with the permeability $\kappa$ defined as

$$\kappa = \frac{\phi}{8\eta\tau}\frac{\left\langle (r_i+\delta)^4\right\rangle}{\langle r_i^2\rangle} \tag{S8}$$

which is a generalized version of the Carman-Kozeny equation (Eqs. 4 and 8 in the Letter). Combining Eqs. (S6) and (S8), we find

$$J = -\kappa\frac{\left\langle \Psi_i \times (r_i+\delta)^4\right\rangle}{L\left\langle (r_i+\delta)^4\right\rangle} \tag{S9}$$

which we plot in Fig. S2 using $\kappa = 1.87\times10^{-17}\ \mathrm{m}^2/(\mathrm{Pa.s})$, for two different pore size distributions: first, a peaked distribution around $r_{\mathrm{p}} = 1.7$ nm which is the ideal case considered in the Letter. Second, a gaussian distribution centered on 1.4 nm and with a half-width-at-half-maximum of 0.4 nm, which reproduces the BJH estimates of the pore size distribution (see section I A). As can be seen on Fig. S2, the two distributions reproduce the experimental data very well and differ only in the transition region between regimes ① and ②.

This last remark suggests that the width of the transition region can be used as an indicator of the pore size distribution. For example, the first experimental data point that shows deviation from the Kelvin-Darcy regime ① is the one at $\Psi_{\mathrm{ext}} = -57$ MPa. Using the Laplace equation, this corresponds to the dewetting of a pore of radius $r' = 2\sigma\cos\theta/\Psi_{\mathrm{ext}} = 2.3$ nm, which agrees well with the maximum pore size from the BJH distribution. Similarly, regime ② is reached for the data point at $\Psi_{\mathrm{ext}} = -128$ MPa which corresponds to $r'' = 1.0$ nm.

## III. POROELASTIC TRANSIENTS

Here we evaluate the transient time to reach steady-state when the sample is taken out of water and placed in a sub-saturated atmosphere in order to interpret the results of Fig. 2b in the Letter. Transient flows in rigid porous systems such as porous silicon are governed by the interplay of viscous flow in the pores (characterized by

the permeability $\kappa$) and the elasticity of the fluid-filled medium through its effective compressibility $\chi\,[\mathrm{Pa}^{-1}]$ [1]. Generally, $\chi = (\chi_{\mathrm{liq}}^{-1} + \chi_{matrix}^{-1})^{-1}$ where $\chi_{\mathrm{liq}}$ is the liquid isothermal compressibility and $\chi_{\mathrm{matrix}}$ the solid matrix compressibility.

This interplay results in a poroelastic diffusion-like equation for the pressure (equivalently, liquid potential $\Psi$)

$$\frac{\partial \Psi}{\partial t} = C \frac{\partial^2 \Psi}{\partial x^2} \tag{S10}$$

with $C = \kappa/(\phi\chi)$ the poroelastic diffusivity. Initially, the sample is saturated with water and the liquid potential is zero everywhere. When the sample is placed in a sub-saturated atmosphere, a liquid potential $\Psi(x = L) = \Psi_{\mathrm{ext}}$ is imposed at the edge, while the presence of bulk liquid water in the serpentine reservoir imposes $\Psi(x = 0) = 0$ at all times. The liquid potential profile (equivalently the pressure profile), initially a step function, thus evolves towards a linear steady-state

$$\Psi_{\mathrm{s}}(x) = \Psi_{\mathrm{ext}}\, x/L. \tag{S11}$$

The solution of the diffusion equation with the above boundary conditions and initial state is

$$\Psi(x,t) = \Psi_{\mathrm{s}}(x) + \Psi_{\mathrm{ext}} \left[ \sum_{n=1}^{\infty} (-1)^{n+1} \frac{2}{\pi n} \sin\left(\pi n \frac{x}{L}\right) \exp\left(-\frac{\pi^2 n^2 C t}{L^2}\right)\right]. \tag{S12}$$

The flux at the reservoir level ($x = 0$) can be calculated from Darcy's law $J = -\kappa \partial\Psi/\partial x$, leading after integration to the volume $V(t)$ transferred from the reservoir to the sample and equivalently to the position of the meniscus as a function of time $X(t) = V(t)/a$ where $a$ is the cross-section area of the serpentine channel:

$$X(t) = v\left[t - \frac{L^2}{6C}\left(1 - \xi(t)\right)\right] \tag{S13}$$

with $v = A\kappa|\Psi_{\mathrm{ext}}|/(aL)$ the meniscus steady-state velocity and

$$\xi(t) = 12 \sum_{n=1}^{\infty} (-1)^{n+1} \exp\left(-(\pi n)^2 C t / L^2\right)/(\pi n)^2 \tag{S14}$$

a dimensionless decay function. It follows that all transient responses can be normalized by plotting $X/v$ as a function of $t$, as is done on Fig. 2b in the Letter. We note from Eq. (S14) that the slowest decaying mode is associated with a timescale

$$\tau_{\mathrm{poro}} = \frac{L^2}{\pi^2 C} \tag{S15}$$

In our system, the porous silicon matrix is much more rigid than the water itself, thus we expect the medium elasticity $\chi = (\chi_{\mathrm{liq}}^{-1} + \chi_{matrix}^{-1})^{-1}$ to be dominated by the liquid compressibility, $\chi \simeq \chi_{\mathrm{liq}}$. The results of Fig. 2b show very good agreement with Eqs. (S13) and (S14) when using the bulk value $\chi_{\mathrm{liq}} = 4.5 \times 10^{-10}\,\mathrm{Pa}^{-1}$ of the isothermal compressibility of liquid water to calculate the poroelastic diffusivity $C = \kappa/(\phi\chi) = 9.2 \times 10^{-8}\,\mathrm{m}^2/\mathrm{s}$ (and the poroelastic timescale $\tau_{\mathrm{poro}} = 110$ s from Eq. S15).

This agreement suggests that in addition to the viscous and capillary properties, the bulk elastic properties (compressibility) of water remain the same in the $\sim 3$ nm-diameter pores studied here.

## IV. EXTERNAL MASS TRANSFER

Here we estimate the contribution of external mass transfer in the vapor outside of the sample and show that its role can be neglected. The mass flux in the porous medium follows

$$\left(\frac{\mathrm{d}m}{\mathrm{d}t}\right)_{\mathrm{po}} = \rho\kappa A \frac{-\Psi_{\mathrm{ext}}}{L} \tag{S16}$$

while the mass flux in the external boundary layer in the air in contact with the edge is

$$\left(\frac{\mathrm{d}m}{\mathrm{d}t}\right)_{\mathrm{ext}} = \frac{M\,A\,\mathrm{Sh}\,D_{\mathrm{v,air}}}{H_{\mathrm{p}}\,RT}\left(p_{\mathrm{ext}} - p_{\infty}\right) \tag{S17}$$

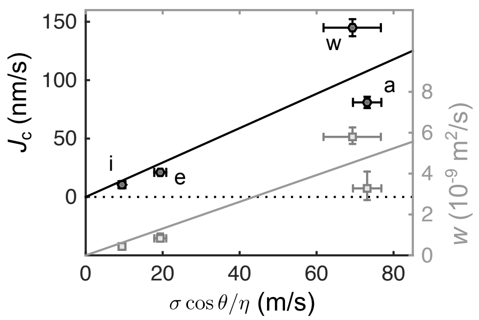


FIG. S3. Plateau-drying ($j_c$) and imbibition responses for different liquids as a function of the driving force $\sigma\cos\theta/\eta$. The lines are a fit giving $\tau = 13$.

where $p_\infty$ refers to the imposed vapor pressure far from the sample, $H_p$ is the thickness of the porous layer, Sh is the Sherwood number characterizing external mass transfer. The vapor pressures are related to the liquid potentials $\Psi_{ext}$ and $\Psi_\infty$ through Kelvin equation.

At steady-state, the two mass fluxes (S16) and (S17) have to be equal, which leads to

$$\frac{p_\infty - p_{ext}}{p_{sat}} = \frac{\ln\left(\frac{p_{ext}}{p_{sat}}\right)}{\beta_{ext}} \tag{S18}$$

where we have defined the dimensionless number

$$\beta_{ext} = \mathrm{Sh}\left(\frac{v_m}{RT}\right)^2 \frac{L\, D_{v,air}\, p_{sat}}{H_p\, \kappa} \tag{S19}$$

In order to estimate the Sherwood number, we consider that evaporation at the edge, which occurs from a long strip, can be approximated as evaporation from a half-cylinder attached to a non-evaporating wall. This geometry can be further approximated as a full cylinder in an infinite domain by the method of images. Using the analogy between heat and mass transfer in the gas phase, we can assume that the Sherwood number for mass transfer is the same as the Nusselt number for heat transfer. A minimum Nusselt number of 0.3 has been evaluated in the literature in geometries similar to ours [6], so that assuming $\mathrm{Sh} > 0.3$ we find $\beta_{ext} > 120$ for our system.

We conclude that the boundary layer mass transfer is not limiting in the overall fluxes and that $\Psi_{ext} = \Psi_\infty$, in other words the water at equilibrium with the edge of the sample is equal to the liquid potential imposed by the relative humidity control far away from the sample.

## V. ALTERNATIVES TO THE MOLECULAR STICKING HYPOTHESIS

In this section, we discuss alternative scenarios to the hypothesis of a negative slip length ($\delta < 0$) of molecular size to explain the observed drying and imbibition dynamics.

From Eqs. $(4-8)$ in the Letter, the plateau-drying and imbibition responses (respectively $j_c$ and $w$) should scale with $\sigma\cos\theta/\eta$ when setting $\delta = 0$. As seen on Fig. S3, the data does not collapse when using this scaling. Furthermore, the tortuosity $\tau = 13$ extracted from the best-fit of the data (lines on Fig. S3) would describe an unlikely convoluted flow path of the liquid in the pores.

Alternatively, an alignment of the data points on Fig. S3 can be obtained by choosing values of the contact angle $\theta$, viscosity $\eta$ or surface tension $\sigma$ that differ from the bulk values listed in table S1. For example, the contact angles can be modified to $\theta = 0$ for water and $\theta = 55°$ for organic liquids. Such values are unlikely since they correspond to a wetting behavior that is opposite to the bulk behavior (organic liquids wet porous silicon significantly better than water). This choice of contact angles would also correspond to a high value of tortuosity, $\tau = 11$.

Increasing the value of viscosity by a factor $\gamma$, on the other hand, allows to keep reasonable values of $\tau$. Choosing $\gamma = 2.5$ for water and $\gamma = 5$ for the organic liquids yields a satisfactory rescaling of the experimental data and a tortuosity $\tau = 3.8$ . While the trend for organic liquids to have a larger viscosity increase under confinement than water is discussed in the literature [7], the choices of $\gamma$ above are arbitrary and not justified by data in the literature.

While $\gamma = 2.5$ for water lies in the upper range of the uncertainty of experimental measurements in the range $0 - 4$ nm [7], the increase of viscosity for organic liquids has been shown to exhibit a very sharp transition to a solid-like behavior [8], which is unlikely to result in an effective value $\gamma = 5$.

Identical results are obtained when *dividing* the surface tensions by the same values of $\gamma$ instead of *multiplying* the viscosities by these factors. This choice, however, is similarly arbitrary, and not supported by literature data which suggest negligible deviations to the bulk values of $\sigma$ above radii of curvature of 1 nm [9].

For the reasons above, we favor the hypothesis of a boundary condition modification in the form of an immobile monolayer of molecules on the pore walls, resulting in a negative slip length $\delta = -d$ which agrees very well with our results as shown in the Letter.

[1] O. Vincent, D. A. Sessoms, E. J. Huber, J. Guioth, and A. D. Stroock, Phys. Rev. Lett. **113**, 134501 (2014).
[2] A. Kovacs, D. Meister, and U. Mescheder, Physica Status Solidi (a) **206**, 1343 (2009).
[3] D. R. Lide, ed., *CRC Handbook of Chemistry and Physics, 90th Edition* (CRC Press, 2009).
[4] F.-M. Pang, C.-E. Seng, T.-T. Teng, and M. Ibrahim, Journal of Molecular Liquids **136**, 71 (2007).
[5] S. Gruener and P. Huber, Phys. Rev. Lett. **100**, 064502 (2008).
[6] F. Stengele and H. Rath, Wärme - und Stoffübertragung **29**, 299 (1994).
[7] U. Raviv, P. Laurat, and J. Klein, Nature **413**, 51 (2001).
[8] J. Klein and E. Kumacheva, Science **269**, 816 (1995).
[9] H. M. Lu and Q. Jiang, *Langmuir*, Langmuir **21**, 779 (2005).
